# Supplementary material for: Identity resolution of software metadata using Large Language Models
Source: arXiv:2505.23500 ancillary file (2025-10-06)

# Supplementary Materials

This document provides additional figures and details supporting the main article: "*Identity resolution of software metadata using Large Language Models*", Eva Martín del Pico<sup>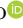</sup>, Josep Lluís Gelpí<sup>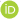</sup> and Salvador Capella-Gutiérrez<sup>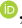</sup>, 2025.

**Table S1:** Model identifiers and provider aliases used during evaluation.

| <b>Model</b>  | <b>Inference API</b> | <b>Exact Identifier / Route Name</b>      |
|---------------|----------------------|-------------------------------------------|
| Mixtral 8x7B  | OpenRouter           | mistralai/mixtral-8x7b-instruct           |
| Mixtral 8x22B | OpenRouter           | mistralai/mixtral-8x22b-instruct          |
| Mistral 7B    | Hugging Face         | mistralai/mistral-7b-instruct-v0.3        |
| Ministral 8B  | OpenRouter           | mistralai/ministral-8b                    |
| Llama 4 Scout | Hugging Face         | meta-llama/Llama-4-Scout-17B-16E-Instruct |
| OpenChat      | OpenRouter           | openchat/openchat-7b                      |
| Llama 3.3     | OpenRouter           | meta-llama/llama-3.3-70b-instruct         |
| GPT-4o        | OpenRouter           | openai/gpt-4o                             |

**Table S2:** Decisions made, accuracy, macro F-1 score, macro precision and macro recall for all evaluated models, including agreement-based proxies. Values are macro-averaged across the three verdict classes (**same**, **different**, **unclear**).

| Model         | Decisions | Accuracy                   | Macro F-1 score            | Macro Precision            | Macro Recall               |
|---------------|-----------|----------------------------|----------------------------|----------------------------|----------------------------|
| Llama 4 Scout | 100       | 0.930 (0.890-0.960)        | 0.611 (0.550-0.649)        | 0.640 (0.626-0.651)        | 0.593 (0.519-0.648)        |
| GPT-4o        | 100       | 0.890 (0.830-0.940)        | 0.581 (0.524-0.627)        | 0.571 (0.515-0.631)        | 0.590 (0.526-0.644)        |
| Llama 3.3     | 100       | 0.810 (0.740-0.880)        | 0.513 (0.458-0.571)        | 0.487 (0.441-0.542)        | 0.571 (0.511-0.620)        |
| Mixtral 8x22B | 100       | 0.840 (0.770-0.900)        | 0.528 (0.467-0.588)        | 0.503 (0.450-0.564)        | 0.569 (0.501-0.627)        |
| Mixtral 8x7B  | 96        | 0.906 (0.865-0.948)        | 0.577 (0.502-0.634)        | 0.607 (0.545-0.646)        | 0.558 (0.479-0.625)        |
| Mistral 7B    | 99        | 0.899 (0.859-0.939)        | 0.571 (0.503-0.626)        | 0.606 (0.547-0.643)        | 0.551 (0.477-0.625)        |
| OpenChat      | 94        | 0.851 (0.798-0.904)        | 0.510 (0.422-0.581)        | 0.558 (0.474-0.627)        | 0.491 (0.412-0.570)        |
| Ministral 8B  | 100       | 0.680 (0.590-0.770)        | 0.420 (0.361-0.479)        | 0.417 (0.371-0.462)        | 0.487 (0.412-0.555)        |
| Proxy I       | 86        | <b>0.965</b> (0.930-1.000) | <b>0.626</b> (0.581-0.667) | <b>0.653</b> (0.640-0.667) | <b>0.607</b> (0.549-0.667) |
| Proxy II      | 85        | 0.963 (0.928-1.000)        | 0.621 (0.569-0.667)        | 0.653 (0.640-0.667)        | 0.599 (0.533-0.667)        |
| Proxy III     | 85        | 0.953 (0.906-0.988)        | 0.609 (0.549-0.653)        | 0.630 (0.576-0.662)        | 0.596 (0.524-0.657)        |
| Proxy IV      | 93        | 0.946 (0.903-0.978)        | 0.591 (0.518-0.640)        | 0.646 (0.632-0.658)        | 0.561 (0.479-0.625)        |
| Proxy V       | 94        | 0.958 (0.926-0.989)        | 0.611 (0.559-0.654)        | 0.651 (0.639-0.662)        | 0.585 (0.521-0.646)        |

**Table S3:** Per-class precision and recall for all evaluated models, including agreement-based proxies. All models, including the proxies, failed to recover any **unclear** cases.

| Model         | P <sub>same</sub>          | R <sub>same</sub>          | P <sub>diff</sub>          | R <sub>diff</sub>          | P <sub>unclear</sub> | R <sub>unclear</sub> |
|---------------|----------------------------|----------------------------|----------------------------|----------------------------|----------------------|----------------------|
| Llama 4 Scout | 0.919 (0.878-0.952)        | 1.000 (1.000-1.000)        | 1.000 (1.000-1.000)        | 0.778 (0.556-0.944)        | 0.000                | 0.000                |
| GPT-4o        | 0.925 (0.887-0.960)        | 0.937 (0.873-0.987)        | 0.789 (0.636-0.944)        | 0.833 (0.667-1.000)        | 0.000                | 0.000                |
| Llama 3.3     | 0.929 (0.892-0.958)        | 0.823 (0.734-0.911)        | 0.533 (0.424-0.682)        | 0.889 (0.722-1.000)        | 0.000                | 0.000                |
| Mixtral 8x22B | 0.932 (0.887-0.973)        | 0.873 (0.797-0.937)        | 0.577 (0.444-0.750)        | 0.833 (0.667-1.000)        | 0.000                | 0.000                |
| Mixtral 8x7B  | 0.905 (0.865-0.939)        | 0.987 (0.961-1.000)        | 0.917 (0.750-1.000)        | 0.688 (0.438-0.875)        | 0.000                | 0.000                |
| Mistral 7B    | 0.895 (0.856-0.939)        | 0.987 (0.962-1.000)        | 0.923 (0.769-1.000)        | 0.667 (0.444-0.889)        | 0.000                | 0.000                |
| OpenChat      | 0.855 (0.814-0.900)        | 0.973 (0.932-1.000)        | 0.818 (0.600-1.000)        | 0.500 (0.278-0.722)        | 0.000                | 0.000                |
| Ministral 8B  | 0.900 (0.841-0.961)        | 0.684 (0.582-0.785)        | 0.350 (0.265-0.455)        | 0.778 (0.556-0.944)        | 0.000                | 0.000                |
| Proxy I       | <b>0.958</b> (0.920-1.000) | <b>1.000</b> (1.000-1.000) | <b>1.000</b> (1.000-1.000) | <b>0.822</b> (0.647-1.000) | <b>0.000</b>         | <b>0.000</b>         |
| Proxy II      | 0.958 (0.919-1.000)        | 1.000 (1.000-1.000)        | 1.000 (1.000-1.000)        | 0.798 (0.600-1.000)        | 0.000                | 0.000                |
| Proxy III     | 0.959 (0.919-1.000)        | 0.986 (0.957-1.000)        | 0.930 (0.786-1.000)        | 0.801 (0.600-1.000)        | 0.000                | 0.000                |
| Proxy IV      | 0.939 (0.895-0.975)        | 1.000 (1.000-1.000)        | 1.000 (1.000-1.000)        | 0.684 (0.438-0.875)        | 0.000                | 0.000                |
| Proxy IV      | 0.953 (0.918-0.987)        | 1.000 (1.000-1.000)        | 1.000 (1.000-1.000)        | 0.756 (0.562-0.938)        | 0.000                | 0.000                |

**Listing S1:** First message in the prompt, containing the instruction template sent to the model. This message was followed by two entry messages, additional messages with metadata and associated URL content, and a final message specifying the expected output format, as described in the Methods section.

### Task: Software Metadata Verification

I am integrating software metadata from multiple sources. I  
    ↪ have two metadata entries that may or may not belong  
    ↪ to the same software.

Your task is to compare one entry against the other and  
    ↪ determine whether they refer to the same tool.

### Input Format

You will receive inputs in **multiple parts**. Each part  
    ↪ may include:

- JSON-formatted metadata for a software tool
- Extracted content from the tool's repository (e.g.,  
    ↪ README files) or webpage (e.g., HTML, project  
    ↪ descriptions). **These contents are provided**  
    ↪ **explicitly because you do not have internet access.**  
    ↪ **Treat all provided content as final and in-scope. Do**  
    ↪ **not assume any external URLs can be accessed.**

The two tools are introduced as:

- "The first software metadata\_entry"
- "The second software metadata\_entry"

### Processing Instructions

1. Compare the metadata of each tool, prioritizing:
  - repository URLs
  - webpages
  - descriptions
  - documentation content (e.g., README)
  - authorship or contact info
  - associated publications or citations
2. **IMPORTANT**: The tool names are often the same across  
    ↪ entries. This is expected and should **not** be used  
    ↪ **alone** to decide if they refer to the same software.
3. Carefully analyze the provided repository or webpage  
    ↪ content. Look for:
  - Link similarity (e.g., GitHub, SourceForge)

- Shared or related descriptions
- Overlapping contributors, emails, or institutions
- Common citations or programming languages
- Usage instructions or tool behavior that match

4. Wait until the final message says:

```

**"All parts have been sent. Please now analyze the
  ↪ entries and provide the output as specified."**

```

Only then should you perform the analysis.

5. Your response must be a Python dictionary with the

- ```

↪ following keys:
- 'verdict': one of "Same", "Different", or
  ↪ "Unclear"
- 'explanation': 2-3 sentences explaining your decision,
  ↪ based only on the provided data
- 'confidence': one of "high", "medium", or "low"
- 'features': a list of metadata features you relied on
  ↪ (e.g., "repo match", "shared authors")

```

Do not use generic templates or placeholder text. Your

```

↪ answer must reflect the actual input.

```

### Output Format

Use this structure for your answer:

```

'''python
{
  "verdict": "<Same | Different | Unclear>",
  "explanation": "<brief reasoning based on the actual
    ↪ data>",
  "confidence": "<high | medium | low>",
  "features": ["<feature1>", "<feature2>", "..."]
}
'''

```

**Figure S1:** Normalized confusion matrices for all evaluated models, along with summary tables showing the distribution of gold standard labels (Table 1) and the number of cases solved by each LLM (Table 2). Rows represent true labels, and columns represent predicted labels.

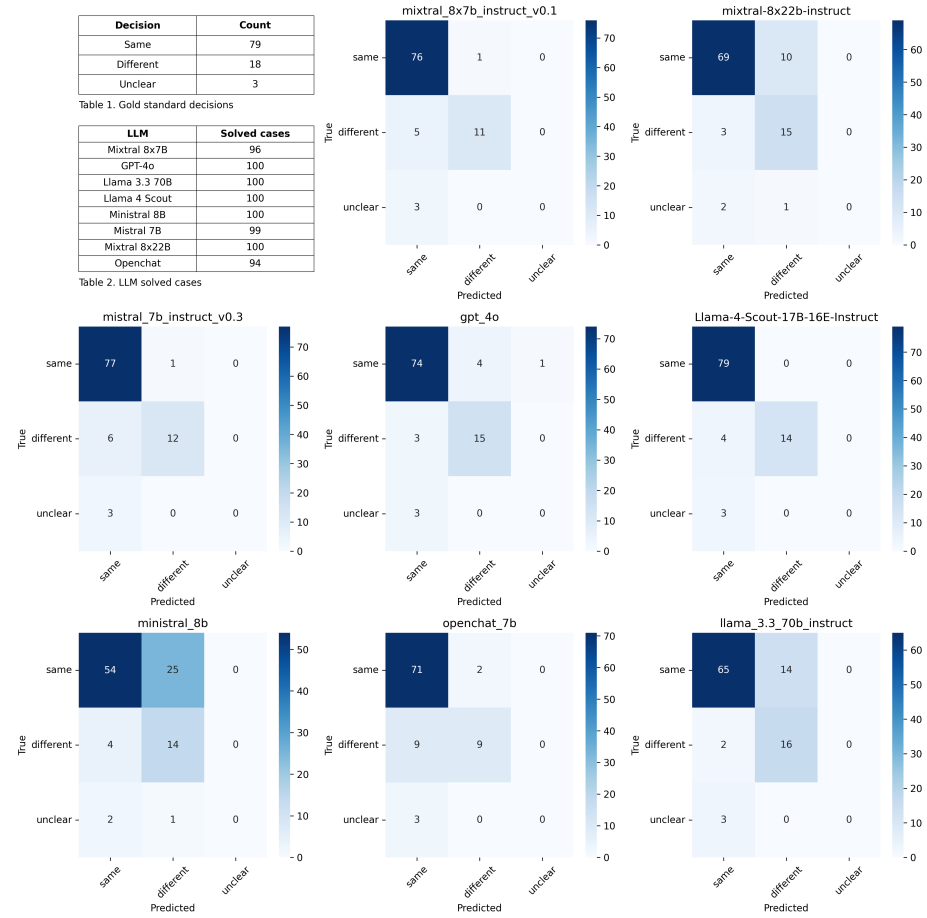

Supplement: Supplementary file 1 [file Supplementary_materials.pdf]
